# Supplementary material for: Direct visualization of polaron formation in the thermoelectric SnSe
Source: arXiv:2111.10012 ancillary file (2021-11-22)
Supplement: Supplementary file 1 [file si.pdf]

# Supplementary information: Direct visualization of polaron formation in the thermoelectric SnSe

Laurent P. René de Cotret[1], Martin R. Otto[1], Jan-Hendrik Pöhls[1,†], Zhongzhen Luo[2], Mercouri G. Kanatzidis[2], Bradley J. Siwick[1,3,*]

[1]Department of Physics, Center for the Physics of Materials, McGill University, Montréal, QC, CA
[2]Department of Chemistry, Northwestern University, Evanston, IL, USA
[3]Department of Chemistry, McGill University, Montréal, QC, CA
[†]Currently at the Department of Chemistry and Chemical Biology, McMaster University, Hamilton, ON, CA
[*]To whom correspondence should be addressed: bradley.siwick@mcgill.ca.

# Contents

**S1 Materials and Methods** **3**

S1.1 Materials . . . . . . . . . . . . . . . . . . . . . . . . . . . . . . . . . . . . . . . 3

S1.2 Methods . . . . . . . . . . . . . . . . . . . . . . . . . . . . . . . . . . . . . . . 3

**S2 Details on ultrafast electron diffuse scattering experiments and data analysis** **5**

S2.1 Ultrafast laser pumping . . . . . . . . . . . . . . . . . . . . . . . . . . . . . . 5

S2.2 Absence of dynamics of the Bragg peak profiles . . . . . . . . . . . . . . . . . 6

S2.3 Diffuse dynamics at high-symmetry points . . . . . . . . . . . . . . . . . . . . 6

S2.4 Comparison of Debye-Waller dynamics along $\mathbf{b}^\star$ and $\mathbf{c}^\star$ . . . . . . . . . . . . . . . . . 6

S2.5 Comparison of diffuse increase along $\mathbf{b}^\star$ and $\mathbf{c}^\star$ . . . . . . . . . . . . . . . . . . . . 6

S2.6 Ultrafast phonon amplitude changes from Bragg intensity . . . . . . . . . . . . 7

S2.7 Energy flow between electrons and zone-center optical modes . . . . . . . . . . 7

S2.8 Upper bound on temperature increase . . . . . . . . . . . . . . . . . . . . . . 8

S2.9 Photocarrier density vs. thermal carrier density . . . . . . . . . . . . . . . . . 8

S2.10Possibility of intervalley scattering . . . . . . . . . . . . . . . . . . . . . . . . 9

S2.11Polaronic contribution to scattering intensity . . . . . . . . . . . . . . . . . . 10

# S1 Materials and Methods

## S1.1 Materials

SnSe ingots (20 g) were synthesized by mixing appropriate ratios of high purity starting materials (Sn chunk, 99.999%, American Elements, USA and Se shot, 99.999%, 5N Plus, Canada) in 13 mm diameter quartz tubes. The tubes were flame-sealed at a residual pressure of $1 \times 10^{-4}$ mmHg, then slowly heated to 1223 K over 10 h, soaked at this temperature for 6h and subsequently furnace cooled to room temperature. The obtained ingots were crushed into powder and flame-sealed in quartz tubes, which were placed into other, bigger, flame-sealed quartz tubes. Crystals with dimensions of ∼13 mm (diameter) × 20 mm (length) were obtained.

Seven samples were used for the ultrafast electron scattering measurements, to ensure reproducibility. Six samples were ultramicrotomed with a diamond blade, while one sample was mechanically exfoliated. Three of the ultramicrotomed samples were cut from a first SnSe mother flake at a thickness of 90 nm. The remaining three ultramicrotomed samples were cut to a thickness of 70 nm from a different mother flake, synthetized separately from the first. The exfoliated sample was prepared from the second mother crystal, with a final thickness of 45 nm. The thickness of the exfoliated samples were estimated based on the ratio of diffracted intensity compared to the ultramicrotomed samples with known thicknesses.

## S1.2 Methods

Ultrafast electron scattering measurements were carried out in a homemade, radio-frequency compressed instrument [52, 55]. A diagram is shown in Figure S1.

Pulses of roughly $1 \times 10^6$ electrons were emitted at 1 kHz. 35 fs pulses of 800 nm light were upconverted to 266 nm and focused in vacuum on a bulk photocathode. Electrons were accelerated in a DC field to a total energy of 90 keV. Electron bunches were compressed with a 3 GHz compression cavity to a time-resolution between 130 fs and 300 fs, depending on the number of electrons per bunch. Electron pulses were focused on a Gatan Ultrascan 895 electron camera. Pump pulses of 800 nm light were

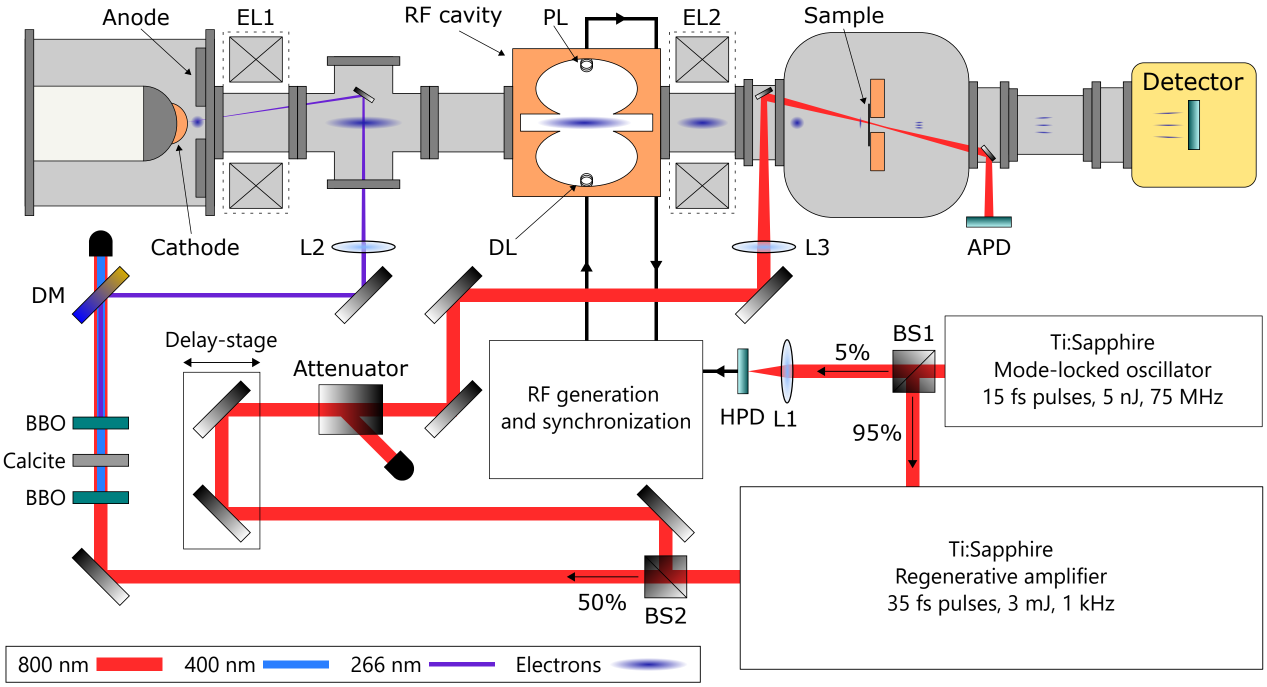


Figure S1: Diagram of the instrument used for ultrafast electron scattering experiments. BS1/2: Beam splitter. HPD: high-bandwidth (>12 GHz) photodiode. BBO: $\beta$-Barium borate crystal. DM: Dichroic mirror. BS1/2: Beamsplitter. L1/2/3: Focusing lens. EL1/2: Electron lens. APD: alignment photodiode. HPD: High-bandwidth photodiode. DL: Driving loop. PL: Pickup loop.

shone on the samples, with a spatial full-width at half-maximum (FWHM) at least thrice as wide as the sample area to ensure uniform photoexcitation.

To minimize the effect of long-term laser power fluctuations on the electron number, data points were acquired at random, until averaging was sufficient. Data acquisition time ranged from 4 h to 72 h, depending on the sample area and the amount of time-points required.

The experimental repetition rate was varied from 25 Hz to 1000 Hz to try and detect any heat accumulation in the sample. However, the dynamics were found to be identical – except for significantly increased noise at lower repetition rates.

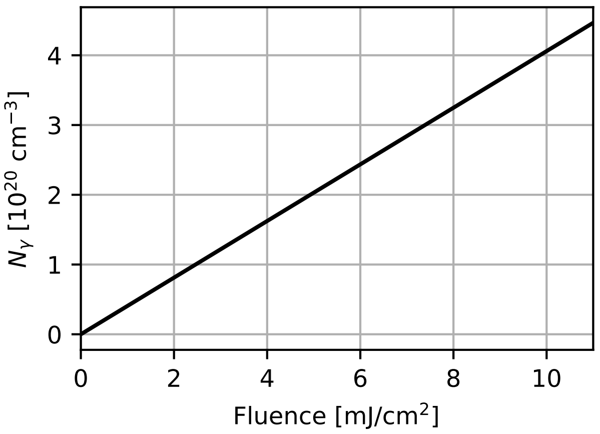


Figure S2: Photocarrier density generated in SnSe for800 nm pump fluences on a 50 µm × 50 µm × 0.045 µm sample.

# S2 Details on ultrafast electron diffuse scattering experiments and data analysis

## S2.1 Ultrafast laser pumping

In this section, we determine the amount of energy that ultrafast laser pumping deposits in the samples used for ultrafast electron diffuse scattering experiments. The total energy deposited for a particular fluence $f$, $E(f)$, is given by

$$E(f) = (1 - R)\eta f \left(1 - e^{-\frac{t}{\delta}}\right) \tag{1}$$

where $R = 0.54$ is the reflectivity at 1.55 eV[54], $\eta = 0.27$ is the internal quantum efficiency[1], $t$ is the sample thickness, and $\delta = 100\,\text{nm}$ is the penetration depth at 800 nm[54, 51]. For reference, roughly 17% of the light is absorbed by a sample with thickness of 45 nm. The photocarrier density $N_\gamma$ is given by $E(f)/V/1.55\,\text{eV}$, where $V$ is the sample volume. The relationship between fluence and $N_\gamma$ is shown in Figure S2 for a 50 µm × 50 µm × 0.045 µm sample.

[1]The quantum efficiency of our samples was determined by B. Dringoli and D. Cooke from McGill University via time-resolved Terahertz spectroscopy, which is unpublished at this time

### S2.2 Absence of dynamics of the Bragg peak profiles

A natural question that arises from Fig. 2 is whether or not the diffuse dynamics close to $\Gamma$ can be explained in terms of Bragg peak profile changes. To confirm that this was not the case, Bragg peaks were fit with a Gaussian profile as shown in Fig. 2c. The full-width at half-maximum was tracked over time-delay. The results are shown in Fig. S3. This figure shows that the dynamics close to the Bragg peaks are distinct from peak broadening.

### S2.3 Diffuse dynamics at high-symmetry points

In this section, we investigate the diffuse intensity dynamics at the in-plane high-symmetry points of the orthorhombic Brillouin zone: $Y$, $Z$, and $T$[56]. The result is shown on Fig. S4, compared to the average diffuse increase across the Brillouin zone shown in Fig. 2d. While the rise amplitude is slightly different for every point, the rise *time* is identical ($3.5 \pm 0.5\,\mathrm{ps}$).

### S2.4 Comparison of Debye-Waller dynamics along $\mathbf{b}^\star$ and $\mathbf{c}^\star$

In-plane reflections can be separated into two categories: the reflections which are nearly parallel to the $\mathbf{c}^\star$ axis, and the reflections which are not. For the reflections which are within $\sim 45°$ degrees of the $\mathbf{c}^\star$ axis, the amplitude of the Bragg peak follows a Debye-Waller suppression with two time-constants $400 \pm 100\,\mathrm{fs}$ and $4 \pm 1\,\mathrm{ps}$. The amplitude of the fast exponential component is maximal for reflections which are exactly parallel to $\mathbf{c}^\star$ (i.e. $(00l)$). For reflections which are not nearly parallel to $\mathbf{c}^\star$ (i.e. $(0k0)$), only the slower time-constant is present. Fig. S5 shows the comparison between the amplitude suppression for reflections which are exactly parallel to $\mathbf{b}^\star$ ($\{(0k0) \mid k \in 2\mathbb{Z}\}$) and reflections which are exactly parallel to $\mathbf{c}^\star$ ($\{(00l) \mid l \in 2\mathbb{Z}\}$).

### S2.5 Comparison of diffuse increase along $\mathbf{b}^\star$ and $\mathbf{c}^\star$

Analogously to the previous section, we can compare the scattering intensity change near zone-center (region (2), Fig. 2b) for reflections which are either parallel to $\mathbf{b}^\star$ or $\mathbf{c}^\star$. The result are shown in Fig. S6. Note that the data presented in Fig. S6 is *raw*; nearby Bragg peak contribution was not

subtracted.

## S2.6 Ultrafast phonon amplitude changes from Bragg intensity

The calculation of vibrational amplitude increase with respect to fluence from Fig. 5 is presented in this section. The time-resolved suppression of Bragg intensity due to atomic vibrations is given by the following expression:

$$\begin{aligned}\frac{I_0(\mathbf{q},t)-I_0(\mathbf{q},0)}{I_0(\mathbf{q},0)} &\equiv \Delta I_0(\mathbf{q},t)\\ &= \frac{N_c I_e |F|^2}{N_c I_e |F|^2}\frac{\left[e^{-2M(\mathbf{q},t)}-e^{-2M(\mathbf{q},0)}\right]}{e^{-2M(\mathbf{q},0)}}\\ &= e^{-2[M(\mathbf{q},t)-M(\mathbf{q},0)]}-1 \end{aligned} \tag{2}$$

For small displacements, we can use the harmonic potential approximation[59]:

$$-\frac{1}{2}\ln\left[1+\Delta I_0(\mathbf{q},t)\right] = \frac{1}{2}|\mathbf{q}|^2\Delta\langle u^2\rangle \tag{3}$$

Therefore, the expression for the change in mean-square-displacement is:

$$\Delta\langle u^2\rangle = -\frac{\ln\left[1+\Delta I_0(\mathbf{q},t)\right]}{|\mathbf{q}|^2} \tag{4}$$

and the associated error $\sigma_u$ is given by:

$$\sigma_u = \frac{\partial\Delta\langle u^2\rangle}{\partial I}\sigma_I = \frac{-\sigma_I}{|\mathbf{q}|^2\left[1+\Delta I_0(\mathbf{q},t)\right]} \tag{5}$$

where $\sigma_I$ is the uncertainty in the pre-time-zero intensity $I$.

## S2.7 Energy flow between electrons and zone-center optical modes

In this section, we explain how we determine that by 1 ps, most ($>85\%$) of the energy deposited by the laser pump shots have been converted to atomic displacement associated with **c**-polarized strongly-coupled phonons.

The equilibrium mean-square displacement (MSD) of atoms $\langle u^2\rangle_{\text{therm}}$ is given by:

$$\langle u^2\rangle_{\text{therm}}(T) = \frac{6\hbar^2}{\mu k_B\theta_D}\left[\frac{1}{4}+\frac{T}{\theta_D}\int_{s=0}^{\theta_D/T} ds\,\frac{s}{e^s-1}\right] \tag{6}$$

where $\mu$ is the average atomic mass, and $\theta_D = 220\,\mathrm{K}$[60] is the Debye temperature. Since experiments were carried out at 300 K, the total MSD after photoexcitation, $\langle u^2\rangle(\tau)$, is given by:

$$\langle u^2\rangle(\tau) = \langle u^2\rangle_{\mathrm{therm}}(T = 300\,\mathrm{K}) + \Delta\langle u_c^2\rangle(\tau) \tag{7}$$

where $\Delta\langle u_c^2\rangle(\tau)$ is shown in Fig. 5 of the main text. A temperature-equivalent can be assigned to the measurements. A temperature equivalent can be assigned to the measurements $\langle u^2\rangle(\tau)$ via Eq. 6. For example, for a photoexcitation of $13.2\,\mathrm{mJ\,cm^{-2}}$, $\langle u^2\rangle(\tau = 1\,\mathrm{ps}) = \langle u^2\rangle_{\mathrm{therm}}(T = 375\,\mathrm{K})$.

Finally, the excess energy in the carriers was calculated in Sec. S2.1. The excess energy above the band gap (1.55 eV - 0.9 eV) can be converted to a temperature via the heat capacity which is given by [60]. For example, at a fluence of $13.2\,\mathrm{mJ\,cm^{-2}}$, the electrons have enough energy above the conduction band minimum to heat up the sample to 380 K. The ratio between the temperature-equivalent of the MSD and energy deposited by photopumping gives the proportion of energy transferred between photogenerated carriers and strongly-coupled $c$-polarized zone-center phonon modes by 1 ps.

## S2.8 Upper bound on temperature increase

We can estimate an upper bound for the temperature of the material once energy has been deposited, to ensure that our SnSe samples are not transitioning to the *Cmcm* phase during measurements. The Debye temperature of SnSe is 220 K [60], and therefore at room temperature we are comfortably in the high-temperature limit. The heat capacity of SnSe is $52\,\mathrm{J\,mol^{-1}\,K^{-1}}$[60]. For the maximum fluence investigated in this work ($13.2\,\mathrm{mJ\,cm^{-2}}$), the corresponding temperature increase is capped at 229 K *at late times.*

## S2.9 Photocarrier density vs. thermal carrier density

We can compare the photocarrier density with expected thermal carrier density to compare photoexcitation densities to effective electronic temperatures. The effective carrier density, $n_0$, is given by:

$$n_0 \approx 2\left(\frac{2\pi m_e^* k_B T}{h^2}\right)^{\frac{3}{2}} \exp\left(-\frac{E_g}{2k_B T}\right) \tag{8}$$

where $m_e^*$ is the effective electron mass, $k_B$ is the Boltzmann constant, $T$ is the temperature, $h$ is Planck's constant and $E_g$ is the semiconducting gap ([58], §2.6.2.2).

### S2.10 Possibility of intervalley scattering

The isotropic slow rise of diffuse intensity for large wavevectors is incompatible with intervalley scattering, whereby electrons and holes relax from the local band edge to the global band edge by emitting large wavevector phonons[57]. To understand why, the allowed intervalley relaxation pathways were simulated for electrons and holes; the following explanation focuses on electrons for simplicity. Consider $E(\mathbf{k})$ to be the in-plane electronic dispersion in reciprocal space. An initial electron density-of-states $g^i_{e^-}(\epsilon)$ around local band minima is assumed. Electrons with energy $\epsilon$ can only relax to locations in reciprocal space where the dispersion is lower in energy. This constraint can be expressed using the Heaviside step function $\Theta$, where $\Theta\left\{-g^i_{e^-}(\epsilon)\right\}$ is unity for $\epsilon < g^i_{e^-}(\epsilon)$ and zero otherwise. The number of allowed relaxation pathways $P_{e^-}(\mathbf{k})$ in reciprocal space are therefore given by the cross-correlation between the initial electron density $g^i_{e^-}(\epsilon)E(\mathbf{k})$ and the allowed relaxation pathways $\Theta\left\{-g^i_{e^-}(\epsilon)\right\}E(\mathbf{k})$:

$$P_{e^-}(\mathbf{k}) \propto \int_0^\infty d\epsilon \left[g^i_{e^-}(\epsilon)E(\mathbf{k})\right] \star \left[\Theta\left\{-g^i_{e^-}(\epsilon)\right\}E(\mathbf{k})\right]$$

where $\star$ is the normalized cross-correlation operation with symmetric boundary conditions, which accounts for Umklapp scattering processes. The proportionality constant is chosen so that $P_{e^-}(\mathbf{k}) \leq 1$. Similarly, holes scatter up in energy so that:

$$P_{h^+}(\mathbf{k}) \propto \int_0^\infty d\epsilon \left[g^i_{h^+}(\epsilon)E(\mathbf{k})\right] \star \left[\Theta\left\{g^i_{h^+}(\epsilon)\right\}E(\mathbf{k})\right]$$

where $g^i_{h^+}(\epsilon)$ is the initial holes density-of-states. The results of these calculations are shown in Figure S8. While these calculations are sensitive to the initial density-of-states, note that there are still many regions in reciprocal space where relaxation is forbidden regardless of the initial conditions (i.e. $P_{e^-}(\mathbf{k})$ and $P_{h^+}(\mathbf{k})$ are zero). It follows that intervalley scattering of charge-carriers does not explain the isotropic rise in diffuse intensity on a 3.5 ps time-scale.

### S2.11 Polaronic contribution to scattering intensity

The following derivation is based on the work by Guzelturk *et al.* [53] Consider the classical result of electron scattering at zero-temperature:

$$f^0(\mathbf{q}) = \sum_j f_{e,j}(\mathbf{q}) e^{-i\mathbf{q}\cdot\mathbf{r}_j} \tag{9}$$

where $\mathbf{q}$ is the scattering vector, $f(\mathbf{q})$ is the scattering amplitude (i.e. the diffracted intensity is $I_0 = |f|^2$), $\{f_{e,j}\}$ are the atomic form factor for electron scattering, and $\{\mathbf{r}_j\}$ are the equilibrium atomic positions. We model a polaron as a *small* atomic displacement field $\mathbf{u}(\mathbf{r})$ centered at $\mathbf{r} = \mathbf{0}$. The scattering amplitude becomes:

$$\begin{aligned} f(\mathbf{q}) &= \sum_j f_{e,j}(\mathbf{q}) e^{-i\mathbf{q}\cdot[\mathbf{r}_j + \mathbf{u}(\mathbf{r}_j)]} \\ &= \sum_j f_{e,j}(\mathbf{q}) e^{-i\mathbf{q}\cdot\mathbf{r}_j} e^{-i\mathbf{q}\cdot\mathbf{u}(\mathbf{r}_j)} \\ &\approx \sum_j f_{e,j}(\mathbf{q}) e^{-i\mathbf{q}\cdot\mathbf{r}_j} \left(1 - i\mathbf{q}\cdot\mathbf{u}(\mathbf{r}_j)\right) \end{aligned} \tag{10}$$

where the last transformation follows from a first order Taylor expansion, since the displacement $|\mathbf{u}|$ is small. We can separate the contribution of a polaron into:

$$\begin{aligned} f(\mathbf{q}) &\approx f^0(\mathbf{q}) + f^p(\mathbf{q}) \\ &\approx f^0(\mathbf{q}) - i\sum_j f_{e,j}(\mathbf{q}) e^{-i\mathbf{q}\cdot\mathbf{r}_j} \left[\mathbf{q}\cdot\mathbf{u}(\mathbf{r}_j)\right] \end{aligned} \tag{11}$$

Now consider that $\mathbf{q} = \mathbf{G} + \mathbf{k}$, where $\mathbf{G}$ is the nearest Bragg peak and $\mathbf{k}$ is restricted to the first Brillouin zone. With these definitions, $\mathbf{G}\cdot\mathbf{u}(\mathbf{r}_j)$ is the dominant contribution to the term $\mathbf{q}\cdot\mathbf{u}(\mathbf{r}_j)$ for the reflections considered in the main text, so we may further simplify:

$$f(\mathbf{q}) \approx f^0(\mathbf{q}) - i\sum_j f_{e,j}(\mathbf{q}) e^{-i\mathbf{q}\cdot\mathbf{r}_j}\ \mathbf{G}\cdot\mathbf{u}(\mathbf{r}) \tag{12}$$

which is the result presented in the main text. As a simple model for polaronic lattice distortions in SnSe, we consider a Gaussian vector displacement field of the form $\mathbf{u}(\mathbf{r}) \propto e^{|\mathbf{r}|^2/r_p^2}\hat{\mathbf{u}}$, where $2\sqrt{2\ln 2}r_p$ is the full-width at half-maximum of the displacement amplitude. Within this model, the scattering

intensity $I(\mathbf{q}) = |f(\mathbf{q})|^2$ is given by:

$$\begin{aligned}
I(\mathbf{q}) &= |4\pi f_e(\mathbf{q})|^2 \left| S(\mathbf{k}) - i\mathbf{G}\cdot\hat{\mathbf{r}}A\sqrt{\pi}r_p e^{-\frac{|\mathbf{k}|^2 r_p^2}{4}} \right|^2 \\
&= |4\pi f_e(\mathbf{q})|^2 \left[ S(\mathbf{k}) - i\mathbf{G}\cdot\hat{\mathbf{r}}A\sqrt{\pi}r_p e^{-\frac{|\mathbf{k}|^2 r_p^2}{4}} \right] \left[ S(\mathbf{k}) + i\mathbf{G}\cdot\hat{\mathbf{r}}A\sqrt{\pi}r_p e^{-\frac{|\mathbf{k}|^2 r_p^2}{4}} \right] \\
&= |4\pi f_e(\mathbf{q})|^2 \left[ S(\mathbf{k})^2 + A^2\pi(\mathbf{G}\cdot\hat{\mathbf{r}})^2 r_p^2 e^{-\frac{|\mathbf{k}|^2 r_p^2}{2}} \right] \\
&= I_0(\mathbf{q}) + |4\pi f_e(\mathbf{q})|^2 \pi r_p^2 e^{-\frac{|\mathbf{k}|^2 r_p^2}{2}} (\mathbf{G}\cdot\hat{\mathbf{r}})^2
\end{aligned} \tag{13}$$

where $S(\mathbf{k})$ is the crystal shape function (which tends towards $\delta(\mathbf{k})$ for an infinite crystal) and $I_0$ is the scattering intensity at zero temperature. It follows that the fractional change in scattering intensity is given by:

$$\begin{aligned}
\frac{I(\mathbf{q}) - I_0(\mathbf{q})}{I_0(\mathbf{q})} &\equiv \frac{\Delta I(\mathbf{q})}{I_0(\mathbf{q})} \\
&\propto \frac{r_p^2 e^{-\frac{|\mathbf{k}|^2 r_p^2}{2}}}{I_0(\mathbf{q})} (\hat{\mathbf{G}}\cdot\hat{\mathbf{r}})^2
\end{aligned} \tag{14}$$

where $\hat{\mathbf{G}}$ is used to denote the unit vector along the $\mathbf{G}$ reflection. Assuming that the scattering intensity without polaronic lattice distortion near reflection $\mathbf{G}$, $I_0(\mathbf{q} = \mathbf{G} + \mathbf{k})$, falls off like $\frac{1}{\mathbf{k}}$:

$$\frac{\Delta I(\mathbf{q})}{I_0(\mathbf{q})} \propto |\mathbf{k}| r_p^2 e^{-\frac{|\mathbf{k}|^2 r_p^2}{2}} (\hat{\mathbf{G}}\cdot\hat{\mathbf{r}})^2 \tag{15}$$

For a uniaxial displacement field, where $\hat{\mathbf{u}} \equiv \hat{\mathbf{c}}$ (i.e. along the crystal $\mathbf{c}$-axis), the term $\mathbf{G}\cdot\hat{\mathbf{c}}$ only contributes for reflections which have a projection along the vector $\mathbf{c}^\star$. In both cases, to a first approximation, the fractional change in scattering intensity is spherically-symmetric across the Brillouin zone (see main text, Fig. 3c and d)

# References


[51] Enue Barrios-Salgado, MTS Nair, and PK Nair. "Chemically deposited SnSe thin films: thermal stability and solar cell application". In: *ECS Journal of Solid State Science and Technology* 3.8 (2014), Q169.

[52] Robert P Chatelain et al. "Ultrafast electron diffraction with radio-frequency compressed electron pulses". In: *Applied Physics Letters* 101.8 (2012), p. 081901.

[53] B. Guzelturk et al. "Visualization of dynamic polaronic strain fields in hybrid lead halide perovskites". In: *Nature Materials* 20.5 (Jan. 2021), pp. 618–623. DOI: 10.1038/s41563-020-00865-5.

[54] Leonardo Makinistian and Eduardo Aldo Albanesi. "On the band gap location and core spectra of orthorhombic IV–VI compounds SnS and SnSe". In: *physica status solidi (b)* 246.1 (2009), pp. 183–191.

[55] M. R. Otto et al. "Solving the jitter problem in microwave compressed ultrafast electron diffraction instruments: Robust sub-50 fs cavity-laser phase stabilization". In: *Structural Dynamics* 4.5 (2017), p. 051101.

[56] Wahyu Setyawan and Stefano Curtarolo. "High-throughput electronic band structure calculations: Challenges and tools". In: *Computational Materials Science* 49.2 (2010), pp. 299–312. ISSN: 0927-0256. DOI: https://doi.org/10.1016/j.commatsci.2010.05.010. URL: http://www.sciencedirect.com/science/article/pii/S0927025610002697.

[57] J Sjakste et al. "Hot electron relaxation dynamics in semiconductors: Assessing the strength of the electron–phonon coupling from the theoretical and experimental viewpoints". In: *Journal of Physics: Condensed Matter* 30.35 (2018), p. 353001.

[58] Bart Van Zeghbroeck. "Principles of semiconductor devices". In: *Colorado University* 34 (2004).

[59] Bertram Eugene Warren. In: *X-ray Diffraction*. Dover Publications, 1990. Chap. 3, pp. 36–37.

[60] Heribert Wiedemeier et al. "Heat capacity measurements of SnSe and SnSe2". In: *Thermochimica Acta* 43.3 (1981), pp. 297–303.

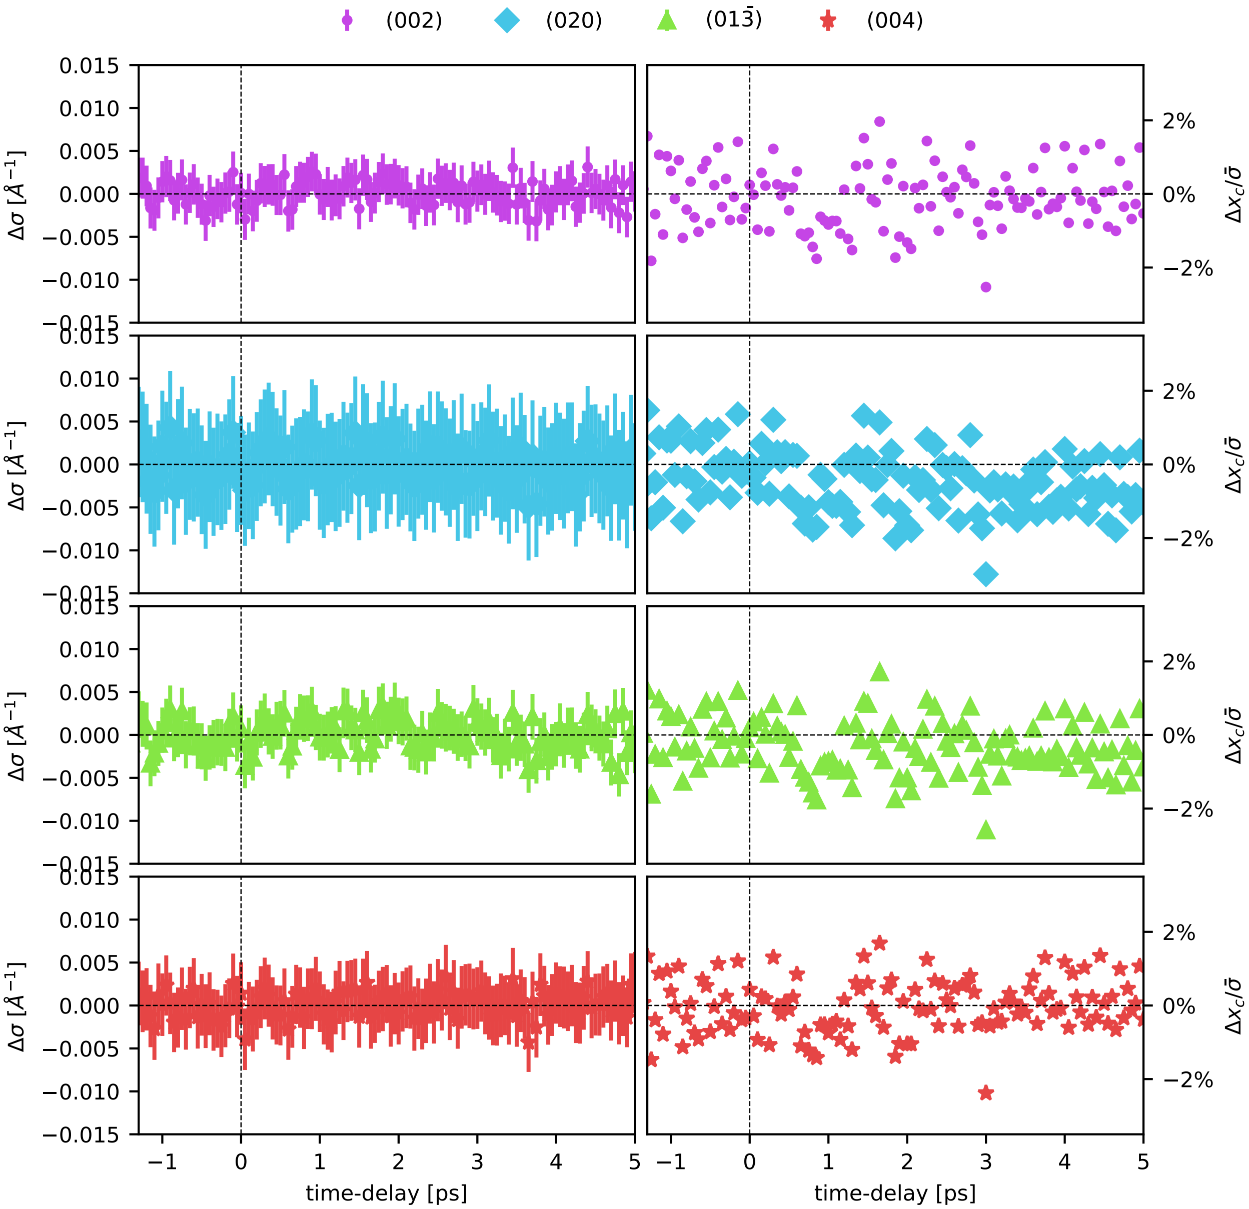


Figure S3: Dynamics of the width and position of various Bragg peaks following photoexcitation. For every time-delay, Bragg peaks were fit with a Gaussian function. In the right column, the change in full-width at half-maximum $\Delta\sigma$ is shown over time. In the left column, the absolute shift in the center position of the peak $\Delta x_c$ is shown, as a percentage of the average full-width at half-maximum $\bar{\sigma}$. For all plots, the error bars represent the covariance of fit parameter.

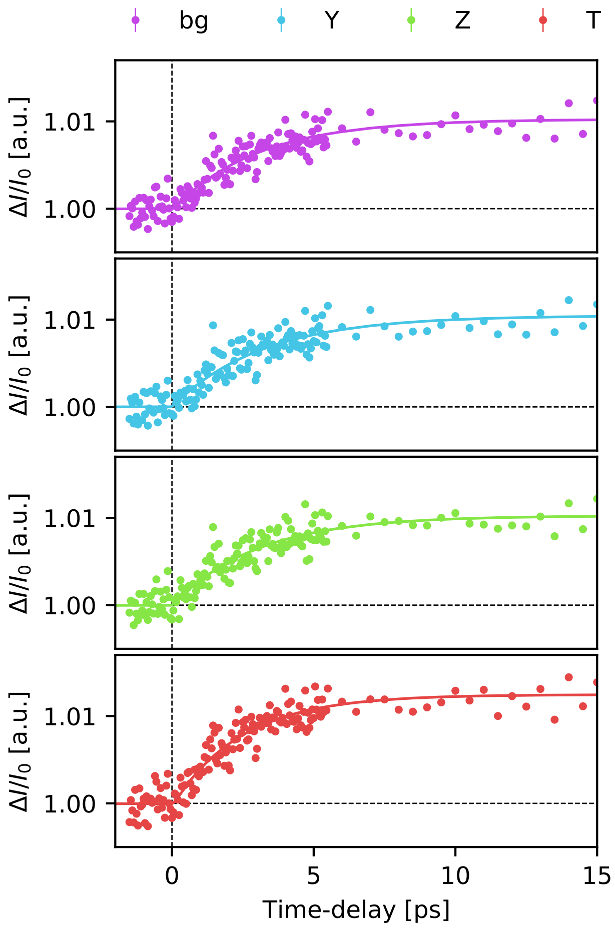


Figure S4: Comparison of diffuse intensity dynamics at the in-plane high-symmetry points of the Brillouin zone $Y$, $Z$, and $T$, compared to the background increase shown in the main text.

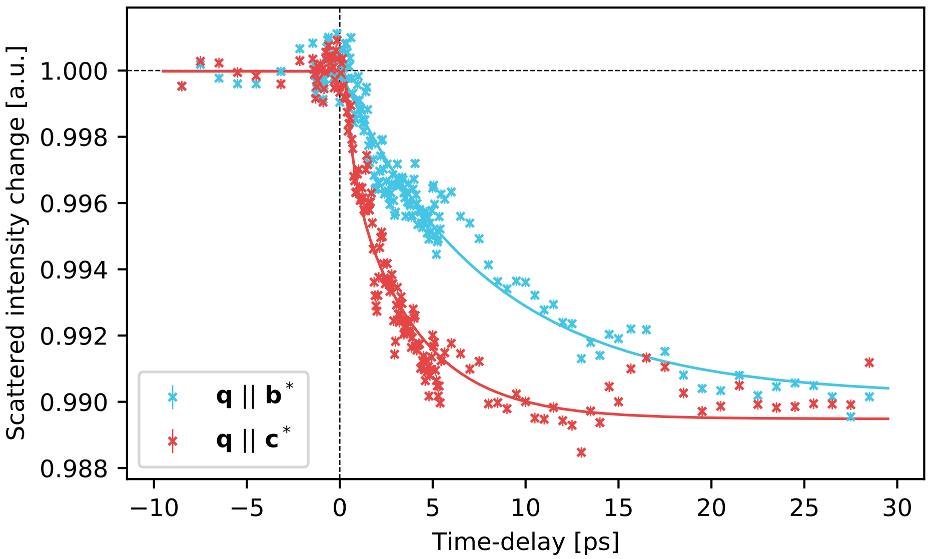


Figure S5: Comparison of the Debye-Waller dynamics in region (1) for reflections exactly parallel to $\mathbf{b}^\star$ ((0$k$0)) and reflections exactly parallel to $\mathbf{c}^\star$ ((00$l$)). Only for reflections parallel to $\mathbf{c}^\star$ are fast dynamics observed.

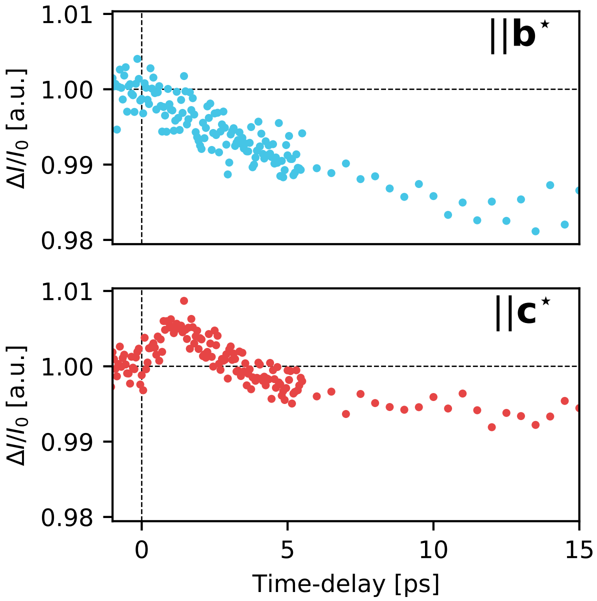


Figure S6: Comparison of the diffuse increase in region (2) for reflections nearly parallel to $\mathbf{b}^\star$ ((031),(040), etc) and reflections nearly parallel to $\mathbf{c}^\star$ ((01$\bar{7}$), (004), etc.). The diffuse dynamics are commensurate with the one-phonon structure factor a transverse mode with polarization along the $\mathbf{c}$ axis.

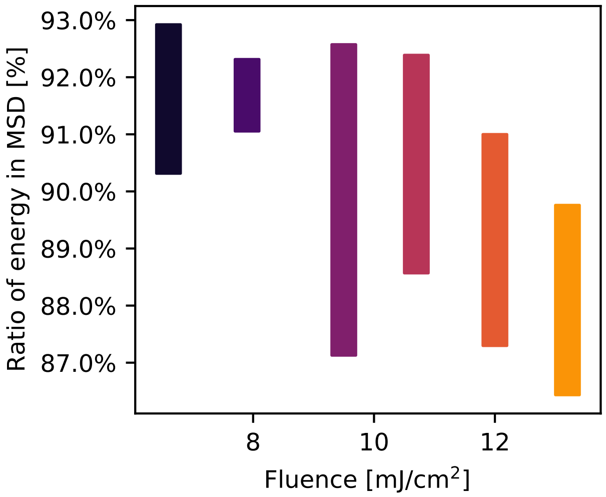


Figure S7: Ratio between the energy deposited by laser pump shots and the energy associated with atomic vibrations due to strongle-coupled, *c*-polarized, zone-center modes at 1 ps for experimental fluences.

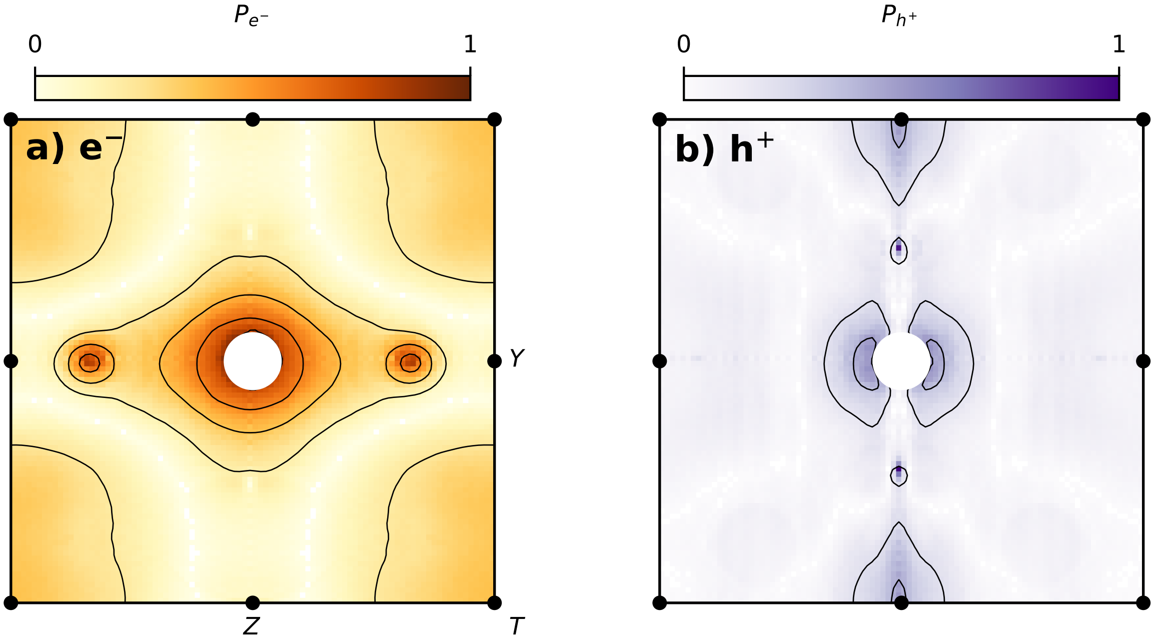


Figure S8: Relative number of allowed relaxation pathways after initial intravalley scattering of charge-carriers. Regions in white represent relaxation pathways that are forbidden, no matter the initial distribution of hot charge carriers. **a** Relative number of relaxation pathways for electrons. **b** Relative number of relaxation pathways for holes.
